# Supplementary material for: Transition between growth of dense and porous films: Theory of dual-layer SEI
Source: arXiv:2112.12628 ancillary file (2022-11-30)
Supplement: Supplementary file 1 [file Supporting_Information.pdf]

# Supporting Information
# Formation of Passivating Dual-Layer Films: Theory of SEI Structure

Lars von Kolzenberg [=1,2], Martin Werres [=1,2], Jonas Tetzloff[3], and Birger Horstmann[*1,2,3]

[1]German Aerospace Center, Pfaffenwaldring 38-40, 70569 Stuttgart, Germany
[2]Helmholtz Institute Ulm, Helmholtzstraße 11, 89081 Ulm, Germany
[3]Ulm University, Albert-Einstein-Allee 47, 89081 Ulm, Germany

November 30, 2022

## 1 Model Parameters

Table SI-1 lists the implemented parameters of our model.

## 2 Experimental Parametrization

To parametrize our model experimentally, we rely on the experiments of Keil *et al.*[4,5], which measure the time and state of charge dependence of capacity fading. In their experiments, Keil *et al.* stored graphite/NMC cells at various states of charge for 9.5 months at 50 °C and subsequently measured the state of health $\mathrm{SoH} = Q/Q_{\mathrm{max}}$. Following the procedure of Single *et al.*[6], we subdivide the SoH fade $\Delta\mathrm{SoH}$ into a linear, non SEI-related capacity loss $\Delta\mathrm{SoH}_{\mathrm{lin}} = 4.5\%$ and an SEI related capacity loss $\Delta\mathrm{SoH}_{\mathrm{SEI}}$, which results from our model with Equation SI-1

$$\Delta\mathrm{SoH}_{\mathrm{SEI}} = \frac{2eA_{\mathrm{el}}}{a^3 Q_{\mathrm{max}}}\bar{L}. \tag{SI-1}$$

Here, $A_{\mathrm{el}} = 14.34\,\mathrm{m}^2$ is the electrode active surface and $Q_{\mathrm{max}} = 10\,080\,\mathrm{C}$ the maximum capacity[4–6].

[=]These authors contributed equally to this work
[*]Corresponding Author: birger.horstmann@dlr.de

| Variable | Description | Value | Source |
|---|---|---|---|
| $e$ | Elementary charge | $1.602 \times 10^{-19}$ C | |
| $k_\mathrm{b}$ | Boltzmann constant | $1.381 \times 10^{-23}$ J K$^{-1}$ | |
| $N_\mathrm{A}$ | Avogadro constant | $6.022 \times 10^{23}$ mol$^{-1}$ | |
| $T$ | Temperature | 298.15 K | |
| $a$ | SEI molecule edge length | 5.42 Å | [1] |
| $\sigma$ | SEI surface energy | 10 mV | |
| $U_0$(SoC) | Graphite OCV curve | Figure SI-1a) | [2] |
| $D$ | Li atom diffusivity inside the SEI | $1 \times 10^{-15}$ m$^2$ s$^{-1}$ | |
| $c_\mathrm{ref}$ | Reference concentration of Li atoms inside the SEI | 0.01 mol m$^{-3}$ | Figure SI-1b) |
| $r_0$ | Rate constant | $5 \times 10^3$ mol m$^{-2}$ s$^{-1}$ | Figure SI-1b) |
| $E_0$ | SEI formation potential | 0.8 V | [3] |
| $E_1$ | SEI energy barrier | 10 mV | |
| $L_0$ | Initial SEI thickness | 0.1 monolayer | |

Table SI-1: Model parameters

Figure SI-1 compares our model predictions with the storage experiments of Keil *et al.*[4,5]. We obtain a good accordance with the experiments, by choosing $c_\mathrm{ref} = 0.01\,\mathrm{mol\,m^{-3}}$ and $r_0 = 5 \times 10^3\,\mathrm{mol\,m^{-2}\,s}$ based on an initial SEI thickness of $h_0 = 15\,\mathrm{nm}$, see Table SI-1. Additionally, the reaction rate $r_0$ affects the transition to porous growth and the chosen value shifts this transition to the experimentally observed regime[7–9].

Figure SI-2 shows the influence of the exchange current density of SEI formation $r_0$ on the onset of porous growth $t_\mathrm{onset}$, defined as the time where instability criterion of Equation 13 is fulfilled. This parameter can be tuned with additives in order to delay the onset of porous growth by using additives. In principle, also $D \cdot c_\mathrm{ref}$ can be tuned. However, in order to have a a less porous SEI, $D \cdot c_\mathrm{ref}$ has to be increased, leading to more rapid SEI formation and faster capacity fade. Thus we focus on $r_0$. It can be seen, that the onset time scales approximately with the square of the inverse of $r_0$:

$$t_\mathrm{onset} \propto \frac{1}{r_0^2}.$$

This is a direct consequence from the scaling of the dimensionless variables. The dimensionless exponential growth rate $\tilde{s}$ is independent of the parameters $c_\mathrm{ref}$, $D$ and $r_0$. The dimensionless current of homogeneous film growth $\tilde{I}_\mathrm{hom} = \mathrm{d}\tilde{L}_0/\mathrm{d}\tilde{t}$ scales with the inverse of the Damkohler number $\tilde{I}_\mathrm{hom} \propto 1/\mathrm{Da}_\mathrm{II} = Dc_\mathrm{ref}/r_0 a$. While the dimensionless current for a fixed parameter set is approximately a function of the square root of the time $\tilde{I}_\mathrm{hom}(t) \approx \mathrm{const}\sqrt{t}$. Thus, the ratio of times for the dimensionless current to fall below a critical value is can be

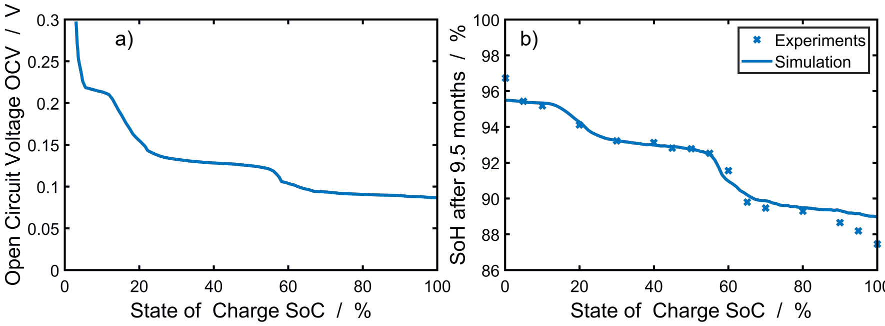


Figure SI-1: a)Graphite open circuit potential $U_0$ depending on the state of charge SoC[6]. b) Comparison of our model predictions (solid line) with the experiments of Keil *et al.*[4,5] (x) for an initial SEI thickness $L_0 = 15\,\text{nm}$.

deduced:

$$\tilde{I}_{\text{hom},1}(t_1) = \tilde{I}_{\text{hom},2}(t_2)$$
$$\Leftrightarrow \text{const} \cdot r_1\sqrt{t_1} = \text{const} \cdot r_2\sqrt{t_2}$$
$$\Leftrightarrow \frac{t_1}{t_2} = \frac{r_2^2}{r_1^2}\ .$$

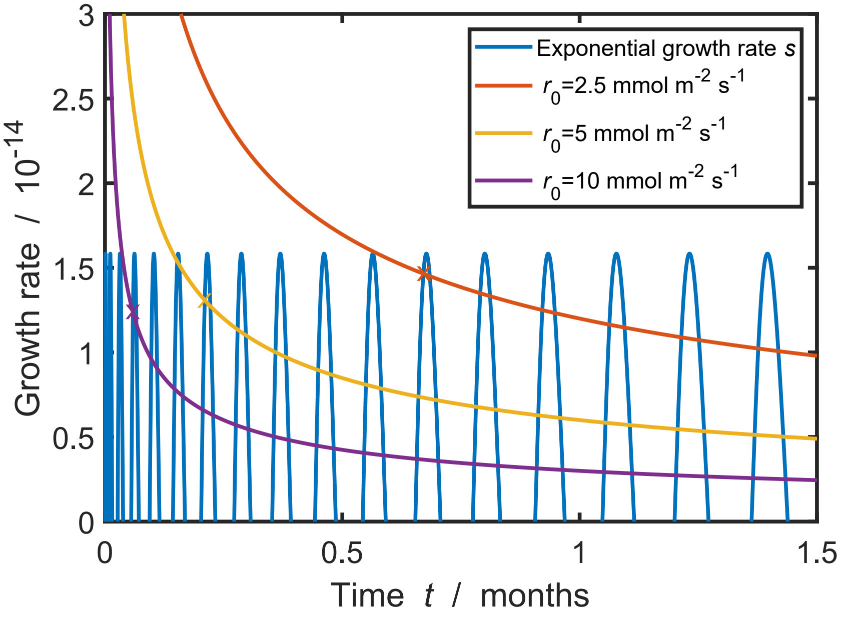


Figure SI-2: Influence of the exchange current density of electrolyte reduction $r_0$ on the onset of unstable SEI growth for SoC=60%. The blue curve indicates the left hand side of Equation 13 and the purple, yellow and red curves the right hand side of Equation 13 for different values of $r_0$. The intersections of the curves correspond to the transition from stable, *i.e.* dense, to unstable, *i.e.* porous, growth.

# 3 Literature Comparison

In the following, we compare the predictions of our model with existing SEI growth models. We choose the SEI model of Single *et al.*[6], because it also describes the potential dependent SEI growth during storage with the following Equation

$$L(t) = \sqrt{c_{\mathrm{ref}} D a^3 \exp\left(-eU_0/k_{\mathrm{B}}T\right) \cdot t + L_0^2}. \tag{SI-2}$$

Figure SI-3 compares the SEI growth predicted by our morphology model with the predictions of the literature model, Equation SI-2[6]. We observe that initially both models coincide, but start to deviate for longer storage times. This effect is more pronounced for lower states of charge.

The observed trend results from the increasing heterogeneity captured by our morphology model. Initially, the SEI grows homogeneous and our model simplifies to the homogenized approach of Single *et al.*[6]. With decreasing SEI current, *i.e.* longer storage times or smaller SoCs, growth becomes more heterogeneous. In this case, our morphology model deviates from the homogeneous

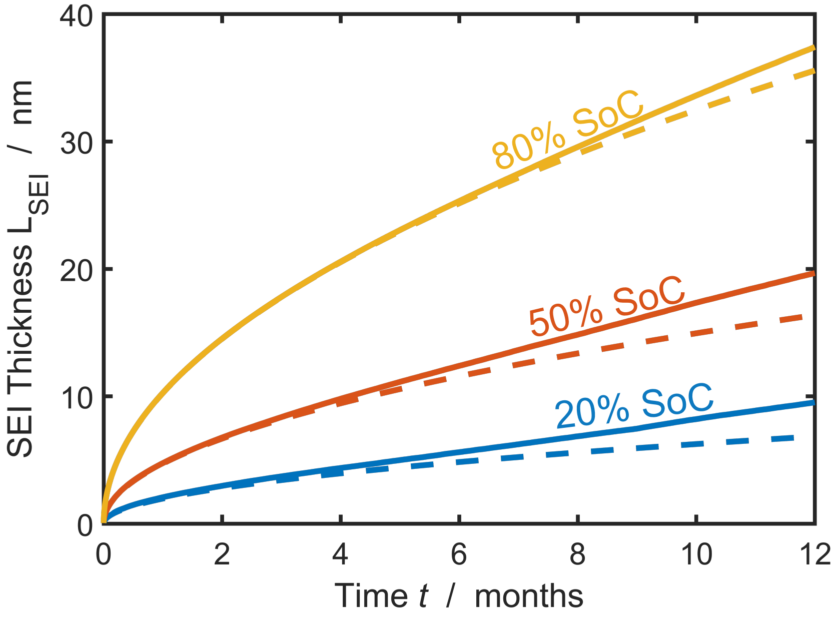


Figure SI-3: Comparison of our morphology model predictions (solid lines) with the homogeneous SEI growth model of Single *et al.*[6] (dashed lines) for three different storage states of charge.

solution and we observe the trend, which is also captured in Figure 2 of our manuscript.

## References


[1] Borodin O, Smith GD, Fan P. Molecular dynamics simulations of lithium alkyl carbonates. J Phys Chem B. 2006;110(45):22773-9.

[2] Birkl CR, McTurk E, Roberts MR, Bruce PG, Howey DA. A Parametric Open Circuit Voltage Model for Lithium Ion Batteries. J Electrochem Soc. 2015;162(12):A2271-80.

[3] Luchkin SY, Lipovskikh SA, Katorova NS, Savina AA, Abakumov AM, Stevenson KJ. Solid-electrolyte interphase nucleation and growth on carbonaceous negative electrodes for Li-ion batteries visualized with in situ atomic force microscopy. Sci Rep. 2020;10(1):1-10.

[4] Keil P, Schuster SF, Wilhelm J, Travi J, Hauser A, Karl RC, et al. Calendar Aging of Lithium-Ion Batteries. J Electrochem Soc. 2016;163(9):A1872-80.

[5] Keil P, Jossen A. Calendar Aging of NCA Lithium-Ion Batteries Investigated by Differential Voltage Analysis and Coulomb Tracking. J Electrochem Soc. 2017;164(1):A6066-74.

[6] Single F, Latz A, Horstmann B. Identifying the Mechanism of Continued Growth of the Solid–Electrolyte Interphase. ChemSusChem. 2018;11(12):1950-5.

[7] Lu P, Harris SJ. Lithium transport within the solid electrolyte interphase. Electrochem commun. 2011;13(10):1035-7.

[8] Harris SJ, Lu P. Effects of inhomogeneities -Nanoscale to mesoscale -on the durability of Li-ion batteries. J Phys Chem C. 2013;117(13):6481-92.

[9] Lu P, Li C, Schneider EW, Harris SJ. Chemistry, impedance, and morphology evolution in solid electrolyte interphase films during formation in lithium ion batteries. J Phys Chem C. 2014;118(2):896-903.
